# Supplementary material for: Neuro-Argumentative Learning with Case-Based Reasoning
Source: arXiv:2505.15742 source file (2025-05-21)
Supplement: Supplementary file 1 [file aacbr.tex]

An abstract \emph{argumentation framework (AF)}~\citep{DUNG-aa} is a pair $\langle \args, \attacks \rangle$, where $\args$ is a set of arguments and $\attacks \subseteq \args \times \args$ is a binary relation defining \emph{attacks} between arguments. We can visualise an AF as a directed graph with arguments as nodes and attacks as edges.
A set of arguments $E \subseteq \args$ \emph{defends} an argument $\argbeta \in \args$ if for all $\argalpha \attacks \argbeta$ there exists $\arggamma \in E$ such that $\arggamma \attacks \argalpha$.

\emph{Abstract Argumentation for Case-Based Reasoning (AA-CBR)}~\citep{aa-cbr} is a machine learning approach for binary classification in which an argumentation framework is constructed from the training data. Each argument in the resulting AF is built from a single data point and is referred to as a \emph{case}.
A partial order defining a notion of \emph{exceptionality} between data points allows the AF to be constructed utilising defeasible reasoning, wherein each data point is an exception to those they attack. Formally:

\begin{definition}
    \label{def:aa-cbr}
    Let $D \subseteq X \times Y$ be a finite \emph{casebase} of labelled examples where $X$ is a set of \emph{characterisations} and $Y = \{\delta, \bar{\delta}\}$ is the set of possible outcomes. Each example is of the form $(x, y)$. Let $\casedefault$ be the \emph{default argument} with $\delta$ the \emph{default outcome}. Let $N$ be an \emph{unlabelled example} of the form $\casenew$ with $y_{?}$ an unknown outcome.  
    Let $\succcurlyeq$ and $\nsim$ be a partial order and binary relation defined over $X$, respectively. The argumentation framework \af{\xnew} mined from $D$ and $x_N$ is $\langle\args, \attacks\rangle$ in which:
    
    \begin{itemize}
        \item $\args = D \cup \{\casedefault\} \cup \{N\}$
        \item for $\casealpha, \casebeta \in D \cup \{(x_{\delta}, \delta)\}$, it holds that $\casealpha \attacks \casebeta$ iff
              \begin{enumerate}
                  \item $y_{\argalpha} \not = y_{\argbeta}$, and
                  \item One of the following holds:  
                  \begin{enumerate}
                      \item $\xalpha$ is more \emph{exceptional} than $\xbeta$ and there is \emph{minimal} difference between them:
                    \begin{enumerate}
                      \item $\x{\argalpha} \succ \xbeta$ and \label{def:aa-cbr:exceptional}
                      \item $\not\exists \casegamma \in D \cup \{(\x{\delta}, \delta)\}$ with $\ygamma = \yalpha$ and $\xalpha \succ \xgamma \succ \xbeta$; \label{def:aa-cbr:minimality} \hfill
                    \end{enumerate}
                    \item or $\xalpha$ is equivalent to $\xbeta$: 
                    \begin{enumerate}
                      \item $\xalpha = \xbeta$; \label{def:aa-cbr:symmetric-attack}
                  \end{enumerate}
                  \end{enumerate}
              \end{enumerate}
        \item for $\casealpha \in D \cup \{(\x{\delta}, {\delta})\}$, it holds that $N \attacks \casealpha$ iff $\xnew \nsim \xalpha.$
    
    \end{itemize}
    
    \noindent
     Finally, we have AA-CBR$(D, \x{N}) = \delta$ if $\casedefault \in \mathbb{G}$ and $\bar \delta$ otherwise, where $\mathbb{G}$ is the grounded extension of \af{N}. 

\end{definition}

A casebase $D$ is \emph{coherent} iff there are no two cases $\casealpha, \casebeta \in D$ such that $\xalpha = \xbeta$ and $y_{\argalpha} \neq y_{\argbeta}$, and it is \emph{incoherent} otherwise. 

% \todoin{

% \begin{itemize}
%     \itemtodo Spike
% \end{itemize}
% }

% As a result of enforcing minimality between cases (Condition \ref{def:aa-cbr:minimality}), not all arguments will have a path to the default case. These arguments, therefore, do not impact the final classification, even if they have features that may be relevant to the new case. These arguments are \emph{spikes}~\citep{monotonicity-and-noise-tolerance}. Formally:

% \begin{definition}
%     Let $\langle \args, \attacks \rangle$ = \af{\xnew} and $\argalpha \in \args$. $\argalpha$ is a \emph{spike} iff there is no path in $\langle \args, \attacks \rangle$ form $\argalpha$ to $\casedefault$.
% \end{definition}

It is practical to define a notion of \emph{regular} AA-CBR~\citep{monotonicity-and-noise-tolerance} in which the choice of default case is such that $\x{\delta}$ is the least element of $X$ under the partial order $\succcurlyeq$ and a case $\argalpha$ is irrelevant to a new case $\argnew$ if $\argnew$ is not an exception to $\argalpha$. Formally:

\begin{definition} 
\label{def:regular-aacbr}
The AF mined from $D$ and $\xnew$ with default argument $\casedefault$ is \emph{regular} when:
\begin{enumerate}
    \item $\xalpha \nsim \xbeta$ iff $\xalpha \not \succcurlyeq \xbeta$, and
    \item $\x{\delta}$ is the least element of $X$.
\end{enumerate}
\end{definition}
