# Supplementary material for: Neuro-Argumentative Learning with Case-Based Reasoning
Source: arXiv:2505.15742 source file (2025-05-21)
Supplement: Supplementary file 2 [file supported-aacbr.tex]

A \emph{bipolar argumentation framework (BAF)}~\citep{bipolar-framework} extends the argumentation framework with the addition of a \emph{supports} relation. A BAF is represented as $\langle \args, \attacks, \supports \rangle$, where $\args$ and $\attacks$ is defined similarly for the AF and $\, supports \subseteq \args \times \args$ is the support relation.

\subsection{Supported AA-CBR}

We introduce an AA-CBR variant using a bipolar argumentation framework as a stepping-stone between AA-CBR and Gradual AA-CBR. This uses a \emph{supports} relation ensuring that no cases are completely disconnected from the graph. We define supported AA-CBR as follows:

\begin{definition}[Supported AA-CBR]
\label{def:supported-aa-cbr}
The bipolar argumentation framework \baf{\xnew} mined from $D$ and $x_N$ is \mbox{$\langle\args, \attacks, \supports\rangle$} in which:

\begin{itemize}
        \item $\args$ and $\attacks$ is defined as in Definition \ref{def:aa-cbr} and;
        \item for $\casealpha, \casebeta \in D \cup \{(x_{\delta}, \delta)\}$, it holds that $\casealpha \supports \casebeta$ iff
              \begin{enumerate}
                  \item $y_{\argalpha} = y_{\argbeta}$, and
                  \item $\xalpha$ is more \emph{exceptional} than $\xbeta$ and there is \emph{minimal} difference between them:
                  \begin{enumerate}
                  \item $\x{\argalpha} \succ \xbeta$ and
                  \item $\not\exists \casegamma \in D \cup \{(\x{\delta}, \delta)\}$ with $\xalpha \succ \xgamma \succ \xbeta$. \hfill \label{def:supported-aa-cbr:minimality}
                  \end{enumerate}
              \end{enumerate}
\end{itemize}
    
\end{definition}

We leave to future work an exploration of supports in AA-CBR under (non-quantitative) bipolar argumentation semantics~\citep{bipolar-framework}. 

Note that we do not constrain the outcome of $\ygamma$ when defining minimality. This ensures that supports necessarily occur from cases that are otherwise spikes in AA-CBR. We define the notion of \emph{regular} Supported AA-CBR as in \definitionref{def:regular-aacbr} and get the following result:

\begin{proposition}
\label{prop:baf-no-spikes}
The regular \baf{\xnew} mined from $D$ and $\xnew$ contains no spikes.
\end{proposition}

\begin{proof}
    Assume towards contradiction that the regular \baf{\xnew} contains a spike $\casealpha$. Either $\casealpha$ does not attack or support any argument, or $\casealpha$ is in a path that ends with an argument, $\casebeta$ that is not the default case and does not attack or support any argument. In either case, we need only consider the argument that does not support or attack any other argument, so without loss of generality, let $\casegamma$ be this case. If $\casegamma$ has no supports or attacks, then either:
    \begin{enumerate}
        \item there must not exist a case $\casetheta$ such that $\xgamma \succcurlyeq \xtheta$ or;
        \item there does exists a case $\casetheta$ such that $\xgamma \succ \xtheta$ and $\exists \casephi \in (D \cup \{\casedefault\})\setminus\{\casegamma, \casetheta\}$, $\xgamma \succ \xphi \succ \xtheta$.
    \end{enumerate} 
    
    However, case 1) cannot be as we are operating under regular Supported AA-CBR wherein $\forall \x{i} \in \args, \x{i} \succcurlyeq \x{\delta}$ so we reach a contradiction.

    Case 2) says that there is case, $\casephi$ in the casebase that is more minimal than $\casegamma$ that would attack or support $\casetheta$ instead. But then $\casephi$ would become a possible candidate for $\casegamma$ to attack or support. If there is no case more minimal than $\casegamma$ that is more exceptional than $\casephi$ then $\casegamma$ would attack (if $\ygamma \not = \yphi$) or support (if $\ygamma = \yphi$) $\casephi$. If there is such a case, then that instead becomes the candidate for $\casegamma$ to attack or support and we can again apply this reasoning, checking if there is a more minimal case, until no cases are more minimal than $\casegamma$ with respect to the candidate case. In which case $\casegamma$ would attack or support this candidate case, contradicting that $\casegamma$ has no attacks or supports.

    Given that every case must therefore attack or support some other case and, $\x{\delta}$ is the least element of $X$, there must always be a path from any case to the default. Thus, $\casealpha$ cannot be a spike.

\end{proof}

An edge-weighted QBAF is a generalisation of a BAF where we can interpret an edge $(\argalpha, \argbeta) \in \edges$ as an attack if $\edgeweights(\argalpha, \argbeta) < 0$ and a support if $\edgeweights(\argalpha, \argbeta) > 0$. 

Gradual AA-CBR captures Supported AA-CBR, with the resulting QBAF that can be directly interpreted as the BAF derived from Supported AA-CBR when using a trivial base score function and an edge weight function that maps a partial order to 1 or 0. Using the indicator function $\indicator(P) = 1$ if $P$, and $0$ otherwise, we can define this relationship formally as follows:

\begin{theorem}
\label{thm:qbaf-to-baf}
Let $\qbafdn{D}{N} = \langle \args, \edges, \basescore, \edgeweights \rangle$ and \baf{\xnew} $= \langle \args, \attacks, \supports \rangle$.
If $\edgeweightspartial(\xalpha, \xbeta) = \indicator(\xalpha \succcurlyeq \xbeta)$ and $\edgeweightsirrelevant(\xnew, \xalpha) = -\indicator(\xnew \nsim \xbeta)$, then $\attacks~\equiv \{(\argalpha, \argbeta)~|~\edgeweights(\argalpha, \argbeta) < 0 \}$ and $\supports~\equiv \{(\argalpha, \argbeta)~|~\edgeweights(\argalpha, \argbeta) > 0 \}$. 
\end{theorem}

To prove \theoremref{thm:qbaf-to-baf}, we start by proving the following Lemmas. Note that as the range of $\edgeweightspartial$ is $\{0, 1\}$, the ranges of the operation $1 - \edgeweightspartial(\xalpha, \xbeta)$, a multiplication of two applications of $\edgeweightspartial$, or a multiplication of $\edgeweightspartial$ and a $1 - \edgeweightspartial(\xalpha, \xbeta)$ operation will all be $\{0, 1\}$.
\begin{lemma}
    \label{lemma:edge-weight-strict}
    $\edgeweightsstrict(\xalpha, \xbeta) = 1 \Rightarrow \xalpha \succ \xbeta$
\end{lemma}

\begin{proof}
    \begin{itemize}
        \item[] $\edgeweightsstrict(\xalpha, \xbeta) = 1$
        \itemthen $\edgeweightspartial(\xalpha, \xbeta) \cdot (1 - \edgeweightspartial(\xalpha, \xbeta)) = 1$ \hfill (by definition of $\edgeweightsstrict$)
        \itemthen $\edgeweightspartial(\xalpha, \xbeta) = 1$ and $(1 - \edgeweightspartial(\xalpha, \xbeta)) = 1$ \hfill (as the range of the operations is $\{0, 1\}$)
        \itemthen $\edgeweightspartial(\xalpha, \xbeta) = 1$ and $\edgeweightspartial(\xbeta, \xalpha) = 0$
        \itemthen $\xalpha \succcurlyeq \xbeta$ and $\xbeta \not \succcurlyeq \xalpha$ \hfill (as $\edgeweightspartial(\xalpha, \xbeta) = \indicator(\xalpha \succcurlyeq \xbeta)$) 
        \itemthen $\xalpha \succ \xbeta$;
    \end{itemize}
\end{proof}

\begin{lemma}
    \label{lemma:edge-weight-not-strict}
    $\edgeweightsstrict(\xalpha, \xbeta) = 0 \Rightarrow \xalpha \not \succ \xbeta$
\end{lemma}
\begin{proof}
    \begin{itemize}
        \item[] $\edgeweightsstrict(\xalpha, \xbeta) = 0$
        \itemthen $\edgeweightspartial(\xalpha, \xbeta) \cdot (1 - \edgeweightspartial(\xalpha, \xbeta)) = 0$ \hfill (by definition of $\edgeweightsstrict$)
        \itemthen $\edgeweightspartial(\xalpha, \xbeta) = 0$ or $(1 - \edgeweightspartial(\xalpha, \xbeta)) = 0$ \hfill (as the range of the operations is $\{0, 1\}$)
        \itemthen $\edgeweightspartial(\xalpha, \xbeta) = 0$ or $\edgeweightspartial(\xbeta, \xalpha) = 1$
        \itemthen $\xalpha \not \succcurlyeq \xbeta$ and $\xbeta \succcurlyeq \xalpha $ \hfill (as $\edgeweightspartial(\xalpha, \xbeta) = \indicator(\xalpha \succcurlyeq \xbeta)$) 
        \itemthen $\xalpha \not \succ \xbeta$;
    \end{itemize}
\end{proof}

\begin{lemma}
\label{lemma:greater-means-not-equal}
$\edgeweightsstrict(\xalpha, \xbeta) = 1 \Rightarrow \edgeweightsequal(\xalpha, \xbeta) = 0$ 

\end{lemma}
Intuitively, if $\xalpha$ is strictly greater than $\xbeta$ by the partial order, then they cannot be equivalent.
\begin{proof}

\begin{itemize}
    \item[] $\edgeweightsstrict(\xalpha, \xbeta) = 1$
    \itemthen $\edgeweightspartial(\xalpha, \xbeta) \cdot (1 - \edgeweightspartial(\xbeta, \xalpha)) = 1$, \hfill  (by definition of $\edgeweightsstrict$)
    \itemthen $\edgeweightspartial(\xalpha, \xbeta) = 1$ and $(1 - \edgeweightspartial(\xbeta, \xalpha)) = 1$, \hfill (as the range of operations is $\{0, 1\}$)
    \itemthen $\edgeweightspartial(\xalpha, \xbeta) = 1$ and $\edgeweightspartial(\xbeta, \xalpha) = 0$,
    \itemthen $\edgeweightspartial(\xalpha, \xbeta) \cdot \edgeweightspartial(\xbeta, \xalpha) = 0$,
    \itemthen $\edgeweightsequal(\xalpha, \xbeta) = 0$, \hfill (by definition of $\edgeweightsequal$) 
\end{itemize}

\end{proof}
\begin{lemma}
\label{lemma:equal-means-not-greater}
$\edgeweightsequal(\xalpha, \xbeta) = 1 \Rightarrow \edgeweightsstrict(\xalpha, \xbeta) = 0$

\end{lemma}
Intuitively, if $\xalpha$ is equivalent to $\xbeta$ by the partial order, then $\xalpha$ cannot be strictly greater than $\xbeta$.
\begin{proof}
\begin{itemize}
    \item[] $\edgeweightsequal(\xalpha, \xbeta) = 1$
    \itemthen $\edgeweightspartial(\xalpha, \xbeta) \cdot \edgeweightspartial(\xbeta, \xalpha) = 1$, \hfill (by definition of $\edgeweightsequal$)
    \itemthen $\edgeweightspartial(\xalpha, \xbeta) = 1$ and $\edgeweightspartial(\xbeta, \xalpha) = 1$, \hfill (as the range of operations is $\{0, 1\}$)
    \itemthen $\edgeweightspartial(\xalpha, \xbeta) = 1$ and $(1 - \edgeweightspartial(\xbeta, \xalpha)) = 0$,
    \itemthen $\edgeweightspartial(\xalpha, \xbeta) \cdot (1 - \edgeweightspartial(\xbeta, \xalpha)) = 0$,
    \itemthen $\edgeweightsstrict(\xalpha, \xbeta) = 0$, \hfill (by definition of $\edgeweightsstrict$)
\end{itemize}
\end{proof}

\noindent
We can now prove Theorem~\ref{thm:qbaf-to-baf} as follows:
    
\begin{proof}
First, we note that $\edgeweights$ has a range of $\{-1, 0, 1\}$ because $\edgeweightspartial$ has a range of $\{0, 1\}$ and no operations that we apply change this range except for a multiplication by $-1$ so we only need to show the theorem holds when $\edgeweights(\argalpha, \argbeta)$ is 1 or -1\footnote{Note that the addition operation $\edgeweightsminimal(\xalpha, \xbeta, \casebasefilter{\fullcasebase}{ \yalpha})  + \edgeweightsequal(\xalpha, \xbeta) = 1$ does not change the range because by Lemmas~\ref{lemma:greater-means-not-equal} and \ref{lemma:equal-means-not-greater}, only one of the two terms can be 1 whilst the other is 0.}. 
We first consider attacks. The set of attacks $\attacks$ in the \baf{\xnew} is given by \definitionref{def:aa-cbr}. We show that the set $\{(\argalpha, \argbeta)~|~\edgeweights(\argalpha, \argbeta) = -1 \}$ is equivalent to set $\attacks$ generated under Definition~\ref{def:aa-cbr}. 

We have that $\edgeweights(\argalpha, \argbeta) = -1$ if either:
\begin{enumerate}
    \item[1)] $\casealpha = \casenew$ and $\edgeweightsirrelevant(\xalpha, \xbeta) = -1$, or 
    \item[2)] $\yalpha \not = \ybeta$ and $\edgeweightsattacks(\casealpha, \casebeta) = -1$. 
\end{enumerate}

If case 1) holds then $\edgeweightsirrelevant(\xalpha, \xbeta) = -1 = -\indicator(\xalpha \nsim \xbeta)$ and so $\xalpha \nsim \xbeta$ holds as required. If case 2) holds then we have that $\edgeweightsminimal(\xalpha, \xbeta, \casebasefilter{\fullcasebase}{ \yalpha})  + \edgeweightsequal(\xalpha, \xbeta) = 1$. By Lemmas~\ref{lemma:greater-means-not-equal}~and~\ref{lemma:equal-means-not-greater}, we then have that either:

\begin{enumerate}
    \item[2.1)] $\edgeweightsstrict(\xalpha, \xbeta) = 1$ and $\edgeweightsequal(\xalpha, \xbeta) = 0$, or
    \item[2.2)] $\edgeweightsstrict(\xalpha, \xbeta)  = 0$ and  $\edgeweightsequal(\xalpha, \xbeta) = 1$.

\end{enumerate}
 If case 2.1) holds, then we know that $\edgeweightsstrict(\xalpha, \xbeta) = 1$ and $\edgeweightsminimal(\xalpha, \xbeta, \casebasefilter{\fullcasebase}{\yalpha}) = 1$. By $\edgeweightsstrict(\xalpha, \xbeta) = 1$ and Lemma~\ref{lemma:edge-weight-strict} we have that $\xalpha \succ \xbeta$.
We can now show that the minimality condition also holds:

 \begin{itemize}
    \item[] $\edgeweightsstrict(\xalpha, \xbeta) \cdot \prod_{\casegamma \in {\casebasefilter{\fullcasebase}{\yalpha}}} (1 - (\edgeweightsstrict(\xalpha, \xgamma) \cdot \edgeweightsstrict(\xgamma, \xbeta))) = 1$
    \itemthen $\prod_{\casegamma \in {\casebasefilter{\fullcasebase}{\yalpha}}} (1 - (\edgeweightsstrict(\xalpha, \xgamma) \cdot \edgeweightsstrict(\xgamma, \xbeta))) = 1$
    \itemthen $\forall \casegamma \in {\casebasefilter{\fullcasebase}{\yalpha}}, (1 - (\edgeweightsstrict(\xalpha, \xgamma) \cdot \edgeweightsstrict(\xgamma, \xbeta))) = 1 $  \footnote{As $\edgeweightspartial$ can only be 1 or 0 and so $\edgeweightsstrict$ can only be 1 or 0.}
    \itemthen $\forall \casegamma \in {\casebasefilter{\fullcasebase}{\yalpha}}, (\edgeweightsstrict(\xalpha, \xgamma) \cdot \edgeweightsstrict(\xgamma, \xbeta)) = 0 $
    \itemthen $\forall \casegamma \in {\casebasefilter{\fullcasebase}{\yalpha}}, \edgeweightsstrict(\xalpha, \xgamma) = 0$ or $\edgeweightsstrict(\xgamma, \xbeta) = 0$
    \itemthen $\forall \casegamma \in {\casebasefilter{\fullcasebase}{\yalpha}}, \xalpha \not \succ \xgamma$ or $\xgamma \not \succ \xbeta$ \hfill (by Lemma~\ref{lemma:edge-weight-not-strict})
    \itemthen $\forall \casegamma \in {\casebasefilter{\fullcasebase}{\yalpha}},$ not ($\xalpha  \succ \xgamma$ and $\xgamma \succ \xbeta$)
    \itemthen $\not \exists \casegamma \in {\casebasefilter{\fullcasebase}{\yalpha}},$ $\xalpha  \succ \xgamma \succ \xbeta$
    \itemthen $\not \exists \casegamma \in \fullcasebase$ with $\ygamma = \yalpha$ and  $\xalpha  \succ \xgamma \succ \xbeta$ as required.
 \end{itemize}

\noindent
 If case 2.2) holds then we have: 
\begin{itemize}
    \item[] $\edgeweightsequal(\xalpha, \xbeta) = 1$
    \itemthen $\edgeweightspartial(\xalpha, \xbeta) \cdot \edgeweightspartial(\xbeta, \xalpha) = 1$
    \itemthen $\edgeweightspartial(\xalpha, \xbeta) = 1$ and $ \edgeweightspartial(\xbeta, \xalpha) = 1$
    \itemthen $\xalpha \succcurlyeq \xbeta$ and $\xbeta \succcurlyeq \xalpha$
    \itemthen $\xalpha = \xbeta$ as required.
\end{itemize}

\noindent
So the conditions under which $\edgeweightspartial(\xalpha, \xbeta) = -1$ are the same conditions that define the set of attacks, $\attacks$. 

We now consider supports. The set of supports $\supports$ in the \baf{\xnew} is given by \definitionref{def:supported-aa-cbr}. We show that the set $\{(\argalpha, \argbeta)~|~\edgeweights(\argalpha, \argbeta) = 1 \}$ is equivalent to set $\supports$ generated under Definition~\ref{def:supported-aa-cbr}. 
We have that $\edgeweightspartial(\argalpha, \argbeta) = 1$ if $\casealpha \not = \casenew$ and $\yalpha = \ygamma$ and $\edgeweightssupports(\casealpha, \casebeta) = 1$. 
We can show that the conditions under which this holds is the same as for $\supports$ as follows:

\begin{itemize}
    \item[] $\edgeweightssupports(\casealpha, \casebeta) = 1$ 
    \itemthen $\edgeweightsminimal(\xalpha, \xbeta, \fullcasebase) = 1$
    \itemthen $\edgeweightsstrict(\xalpha, \xbeta) \cdot \prod_{\casegamma \in \fullcasebase} (1 - (\edgeweightsstrict(\xalpha, \xgamma) \cdot \edgeweightsstrict(\xgamma, \xbeta))) = 1$
    \itemthen $\edgeweightsstrict(\xalpha, \xbeta) = 1$ and $\prod_{\casegamma \in \fullcasebase} (1 - (\edgeweightsstrict(\xalpha, \xgamma) \cdot \edgeweightsstrict(\xgamma, \xbeta))) = 1$\footnote{As $\edgeweightspartial$ can only return a value between 0 and 1.}
    \end{itemize}
    By Lemma~\ref{lemma:edge-weight-strict} we therefore have that $\xalpha \succ \xbeta$. We now show the minimality condition holds:
\begin{itemize}
    \itemthen $\prod_{\casegamma \in \fullcasebase} (1 - (\edgeweightsstrict(\xalpha, \xgamma) \cdot \edgeweightsstrict(\xgamma, \xbeta))) = 1$ \hfill (by Lemma~\ref{lemma:edge-weight-strict})
    \itemthen $\forall \casegamma \in \fullcasebase$, $(1 - (\edgeweightsstrict(\xalpha, \xgamma) \cdot \edgeweightsstrict(\xgamma, \xbeta))) = 1$
    \itemthen $\forall \casegamma \in \fullcasebase$, $(\edgeweightsstrict(\xalpha, \xgamma) \cdot \edgeweightsstrict(\xgamma, \xbeta)) = 0$
    \itemthen $\forall \casegamma \in \fullcasebase$, $\edgeweightsstrict(\xalpha, \xgamma) = 0 $ or $ \edgeweightsstrict(\xgamma, \xbeta) = 0$
    \itemthen $\forall \casegamma \in \fullcasebase$, $\xalpha \not \succ \xgamma$ or $ \xgamma \not \succ \xbeta$ \hfill (by Lemma~\ref{lemma:edge-weight-not-strict})
    \itemthen $\forall \casegamma \in \fullcasebase$, not ($\xalpha \succ \xgamma$ and $ \xgamma \succ \xbeta$)
    \itemthen $\not \exists \casegamma \in \fullcasebase$, $\xalpha \succ \xgamma \succ \xbeta$ as required.
\end{itemize}

\noindent
So the conditions under which $\edgeweightspartial(\xalpha, \xbeta) = 1$ are the same conditions that define the set of supports, $\supports$. 

\end{proof}
